# Supplementary material for: Modelling hippocampal neurogenesis across the lifespan in seven species
Source: arXiv:1105.0695 ancillary file (2011-05-03)
Supplement: Supplementary file 1 [file SupplementaryMaterial.pdf]

# Supplementary material for: Modelling hippocampal neurogenesis across the lifespan in seven species

Stanley E. Lazic

## Model comparisons

For both the Ki67 and DCX data, the ANOVA model is the best fitting, in the sense of having the highest $R^2$ and log-likelihood; however, this is to be expected since models with more free parameters will fit the data better than models with fewer, and the question is whether these extra parameters provide a significantly better fit (in the traditional significance testing framework), or what is the amount of support for each model relative to other models being considered (in the information-theoretic approach, which is used here; see Burnham and Anderson, 2002 and Anderson, 2008). In this case, other than greater familiarity, the ANOVA model has no advantages (and a number of disadvantages, see Lazic, 2008) over the exponential and Weibull models. The power model was clearly the worst for both the Ki67 and DCX data. This can be seen in the column "Weight" in Table 1, which contains the model probabilities (given the set of models and the data). The weights are interpreted as the probability that the model is the best one. Therefore, a probability of 0.01 for the ANOVA model for the Ki67 data means that there is only a 1% chance that it is the best model relative to the others. The exponential model was the best for the DCX data while Weibull model was the best for the Ki67 data. However, the exponential was preferred for the Ki67 data because the 95% CI for the $\delta$ parameter included one ($\delta = 1.57$, 95% CI = 0.89 to 2.25), which means that the Weibull model can be reduced to the exponential. Observations at earlier and later time points would be needed to better discriminate between these two models.

Table 1: Model comparisons (ranked list) for the decrease in $Ki67^+$ (proliferation) and $DCX^+$ (neurogenesis) cells over time, from Ben Abdallah et al., (2008). The exponential and Weibull models both fit the data well.

| Model | DF | logLik | AICc | ΔAICc | Weight | E.Ratio | $R^2$ |
|---|---|---|---|---|---|---|---|
| **Proliferation:** | | | | | | | |
| 1 Weibull | 6 | -252.21 | 519.54 | 0.00 | 0.62 | 1.00 | 0.954 |
| 2 Exponential | 5 | -254.19 | 520.53 | 0.99 | 0.38 | 1.64 | 0.949 |
| 3 ANOVA | 9 | -251.41 | 528.31 | 8.78 | 0.01 | 80.51 | 0.956 |
| 4 Power | 5 | -259.88 | 531.91 | 12.37 | 0.00 | 485.18 | 0.932 |
| **Neurogenesis:** | | | | | | | |
| 1 Exponential | 5 | -307.47 | 627.02 | 0.00 | 0.59 | 1.00 | 0.902 |
| 2 Weibull | 6 | -306.45 | 627.91 | 0.89 | 0.38 | 1.56 | 0.905 |
| 3 ANOVA | 9 | -304.30 | 633.80 | 6.78 | 0.02 | 29.66 | 0.911 |
| 4 Power | 5 | -311.72 | 635.52 | 8.50 | 0.01 | 70.01 | 0.885 |

DF = number of parameters estimated; logLik = natural log of the likelihood; AICc = Second-order Akaike's information criterion; ΔAICc = difference between AICc for each model and the AICc of the best model; Weight = Akaike weights (Bayesian posterior model probabilities); E.Ratio = evidence ratio

## Parameter estimates

In Table 2, it can be seen that the values for the intercept vary widely between studies, and this is due to different types of labelled cells being measured, the data being expressed differently (e.g. total number of cells versus number of cells per unit area), and differences between species. There is also a large amount of uncertainty in many of these estimates because in some studies, young animals were not used, and therefore there are no data for values close to $t = 0$. The models for some data sets could be simplified by letting the number of cells go to zero in the long run (i.e. removing the $\gamma$ term if it was not significantly different from zero), but this parameter was retained in all the models to make them comparable, and also because it is not possible to test this adequately in studies reporting only means and error bars. The slopes, by comparison, showed greater similarity across studies.

Table 2: Parameter estimates with standard errors for an exponential model based on data from published studies.

| Slope ($\alpha$ ) | Drop ($\beta$ ) | Asymptote ($\gamma$) | Marker | Species | Units | Data | Ref |
|---|---|---|---|---|---|---|---|
| 0.524 (0.06) | 10,700 (657) | 264 (200) | Ki67 | Mouse (C57BL/6) | Total number | R | Ben Abdallah et al., (2010) |
| 0.461 (0.07) | 34,692 (3,471) | 1,418 (398) | DCX | Mouse (C57BL/6) | Total number | R | Ben Abdallah et al., (2010) |
| 0.242 (0.01) | 2,981 (148) | 127 (17) | BrdU | Mouse (C57BL/6) | Total number | S | Wu et al., (2008) |
| 0.428 (0.003) | 27,100 (258) | 164 (7) | DCX | Mouse (C57BL/6) | Total number | S | Wu et al., (2008) |
| 1.040 (0.07) | 5,460 (768) | 12 (4) | Retroviral | Mouse (C57BL/6) | Neurons/HPC | S | Morgenstern et al., (2008) |
| 0.348 (0.11) | 11 (2.3) | <1 (0.55) | HH3 | Mouse (C57BL/6) | Cells/mm$^2$ | S | Rodriguez et al., (2008)† |
| 0.184 (0.1) | 820 (309) | 100 (68) | BrdU | Mouse (C57BL/6) | Total number | S | Kronenberg et al., (2006) |
| 0.876 (0.17) | 11,100 (2,860) | 192 (97) | BrdU | Rat (SD) | Total number | S | Lemaire et al., (2000) |
| 0.969 (0.05) | 27,500 (1,310) | 426 (87) | BrdU | Rat (SD) | Density | S | Koehl et al., (2009) |
| 2.23 (1.0) | 64,896 (76,642) | 2,308 (237) | Ki67 | Rat (SD) | Cells/mm$^3$ | R | Epp et al., (2009)‡ |
| 0.922 (0.12) | 66,900 (9,770) | 5,280 (789) | DCX | Rat (SD) | Cells/mm$^3$ | R | Epp et al., (2009) |
| 0.583 (0.28) | 21,000 (5,100) | 1,120 (1,800) | Ki67 | Rat (wild) | Cells/mm$^3$ | R | Epp et al., (2009) |
| 0.893 (0.16) | 84,900 (14,200) | 3280 (1,360) | DCX | Rat (wild) | Cells/mm$^3$ | R | Epp et al., (2009) |
| 0.400 (0.01) | 417,000 (25,600) | 1,930 (206) | DCX | Rat (F334) | Total number | S | Rao et al., (2006)§ |
| 0.115 (0.027) | 8,740 (600) | 240 (212) | BrdU | Hedgehog | Cells/mm$^3$ | S | Alpar et al., (2010) |
| 0.067 (0.061) | 23,000 (35,000) | 2,400 (1,070) | DCX | Hedgehog | Cells/mm$^3$ | S | Alpar et al., (2010) |
| 0.316 (0.01) | 99,700 (63,200) | 4,240 (871) | BrdU | Tree shrew | Total number | R | Simon et al., (2005) |
| 0.236 (0.09) | 99,100 (24,300) | 8490 (9,520) | Ki67 | Macaque | Total number | S | Jabes et al., (2010) |
| 0.211 (0.06) | 21,400 (3,630) | 160 (590) | BrdU/NeuN | Macaque | Total number | S | Jabes et al., (2010) |
| 0.229 (0.01) | 2700 (580) | NA | BrdU | Marmoset | Total number | R | Leuner et al., (2007) |
| 0.138 (0.01) | 205 (31) | 3.8 (0.5) | DCX | Human | Cells/mm$^2$ | R | Knoth et al., (2010) |

† Males and females combined. ‡ Excluded from further analyses and graphs (outlier and low precision). § First data point (at 4.5 weeks) omitted. R = Raw data available; S = Summary data only available, SD = Sprague-Dawley.

## Correction factor for the number of counted Ki67 cells

The adjustment for the number of counted cells ($n$) was given as $n \times 0.67 \times 0.75$. The 0.67 was taken from a very thorough study by Mandyam et al. (2007), where they showed that when mice were injected with 150 mg/kg of BrdU and killed 24 hours later, approximately 33% of BrdU$^+$ cells were still expressing Ki67. This means that when $n$ Ki67 cells are counted, 33% of them will be from cells that divided yesterday, and 67% will be from cells that divided today. Because the calculations took a single day as a unit of time, $n$ was multiplied by 0.67, which eliminated the over-count.

The other adjustment was made for the fact that the number of counted cells does not necessarily indicate the number of additional cells. For example, if five cells divide, there will be a total of ten cells, but only five additional cells. Thus if all of the cells are pre-mitotic, the correct count will be obtained, and if all of the cells are post-mitotic, there will be a 2-fold over-count, which can be corrected by multiplying the cell count by 0.5. The proportion of cells that are pre- and post-mitotic is not known, and therefore a reasonable estimate would be to multiply the number of counted cells by 0.75, which is the average correction factor if all cells are post-mitotic (0.5) and if all are pre-mitotic (1.0). Therefore, taking the above two considerations into account, to estimate the number of new cells added per day, the number of counted cells ($n$) was multiplied by 0.67 and 0.75.

# Figures: Exponential model fit to all data sets

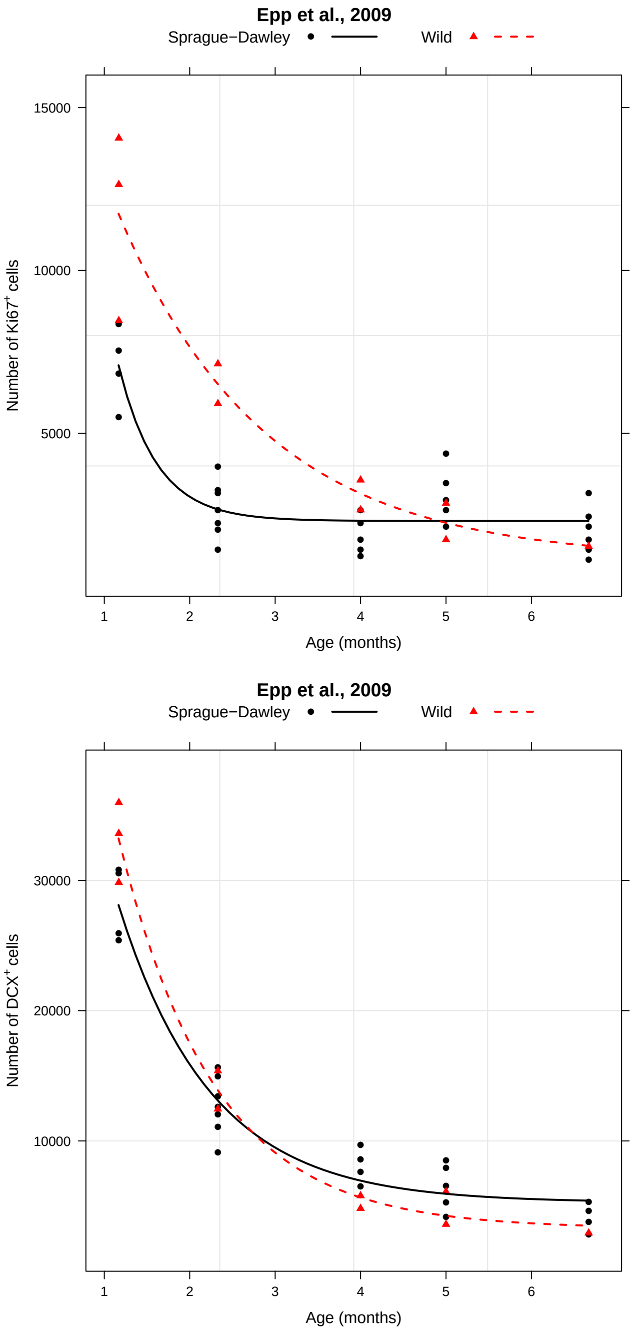


Figure 1:

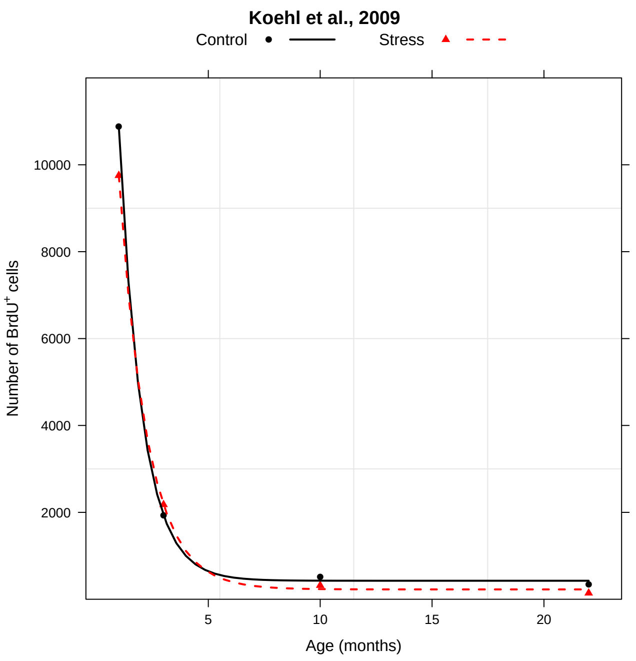


Figure 2:

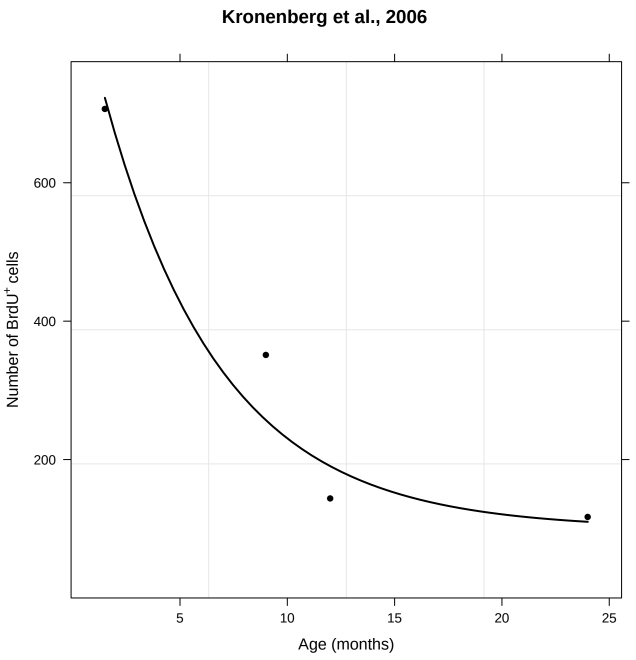


Figure 3:

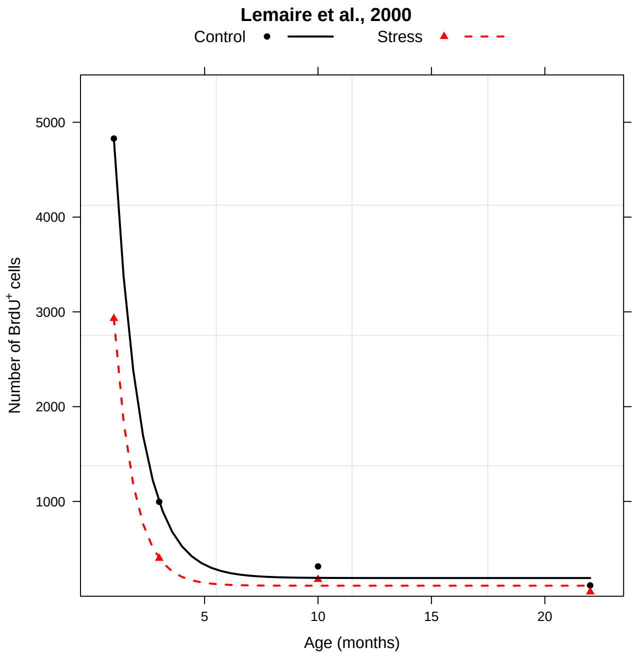


Figure 4:

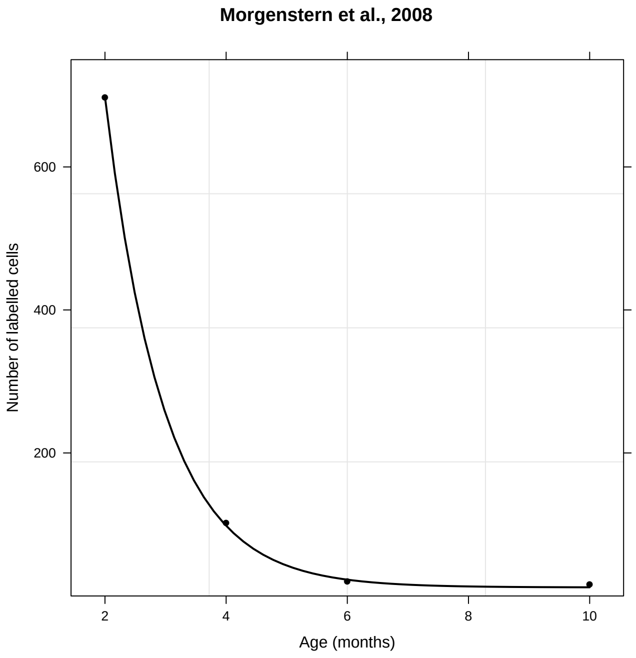


Figure 5:

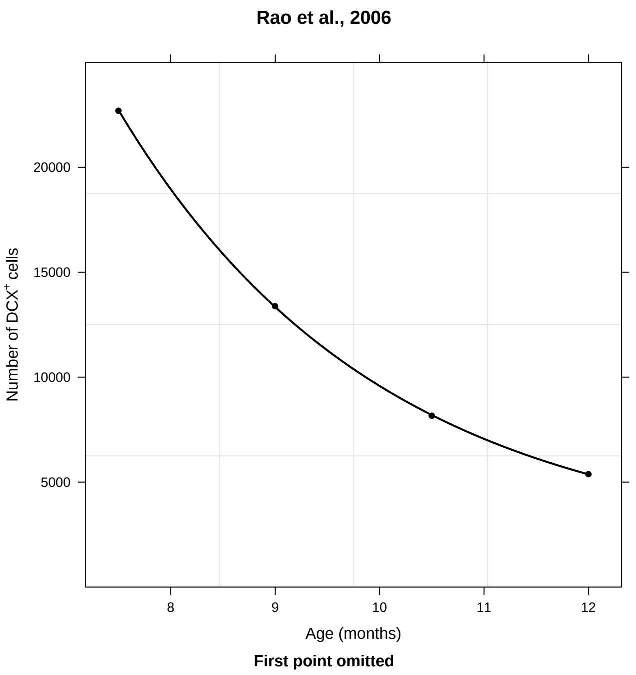


Figure 6:

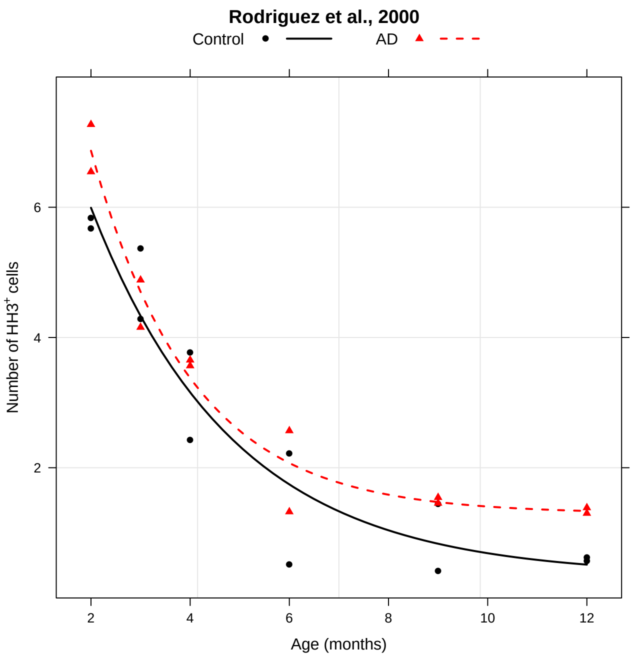


Figure 7:

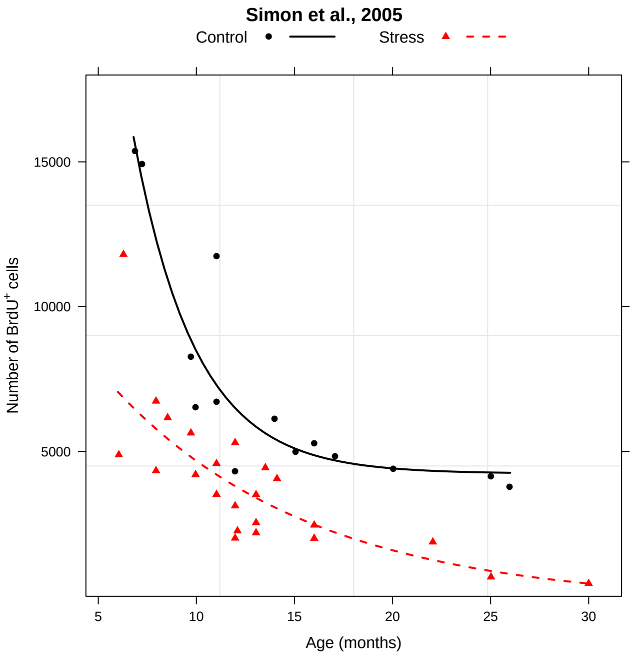
Simon et al., 2005
Control
Stress
15000
10000
5000
Number of BrdU$^+$ cells
5
10
15
20
25
30
Age (months)

Figure 8:

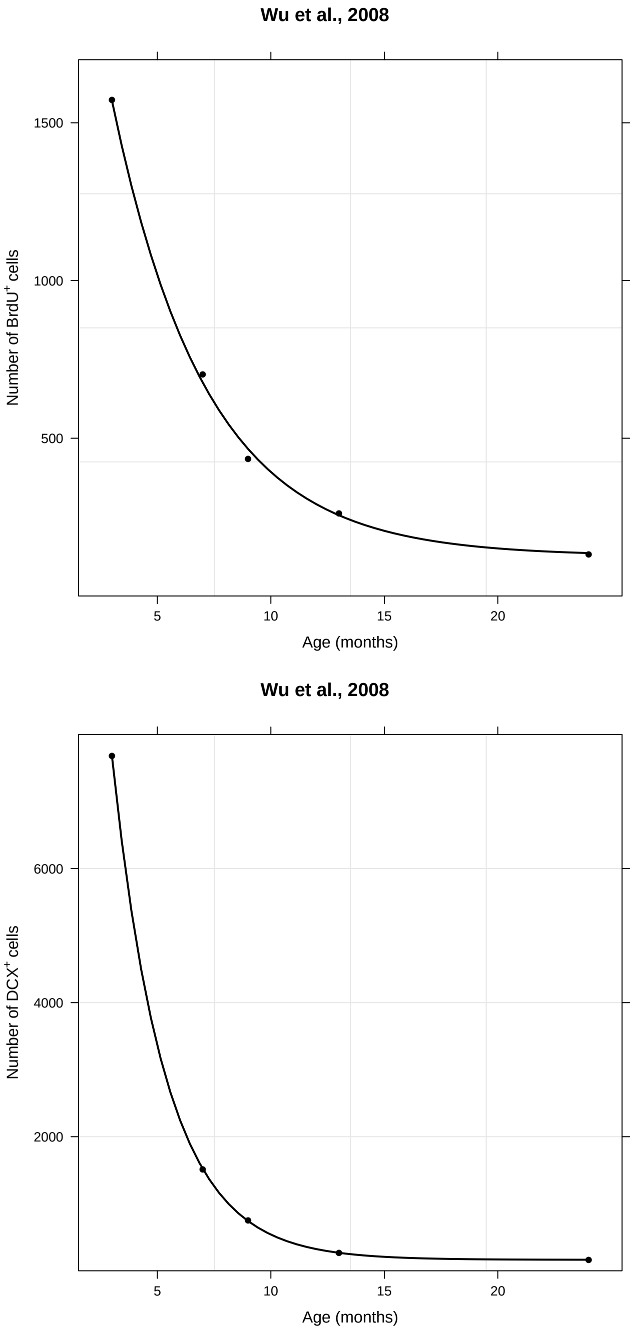
Wu et al., 2008
Number of BrdU+ cells
1500
1000
500
5
10
15
20
Age (months)
Wu et al., 2008
Number of DCX+ cells
6000
4000
2000
5
10
15
20
Age (months)

Figure 9:

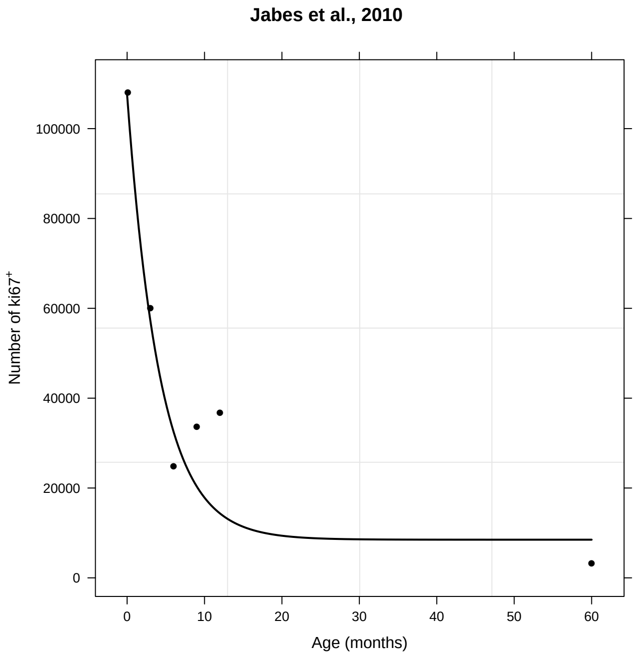
Jabes et al., 2010
Number of ki67+
Age (months)
0
20000
40000
60000
80000
100000
0
10
20
30
40
50
60

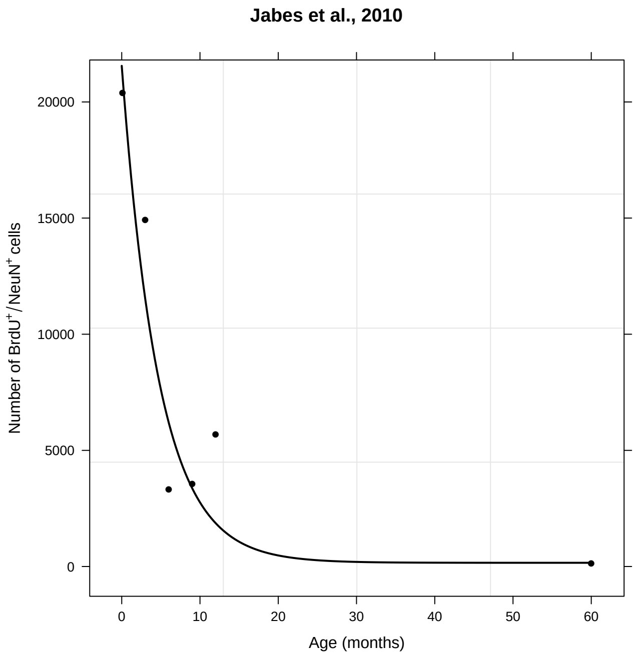
Jabes et al., 2010
Number of BrdU+/NeuN+ cells
Age (months)
0
5000
10000
15000
20000
0
10
20
30
40
50
60

Figure 10:

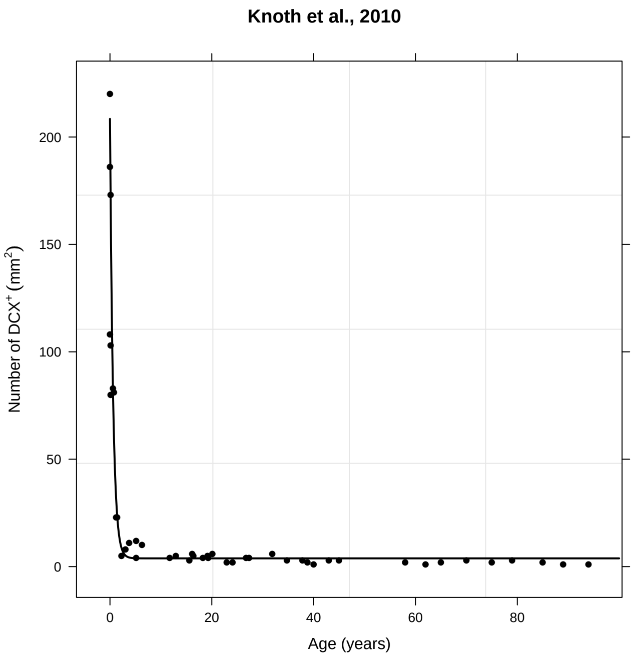


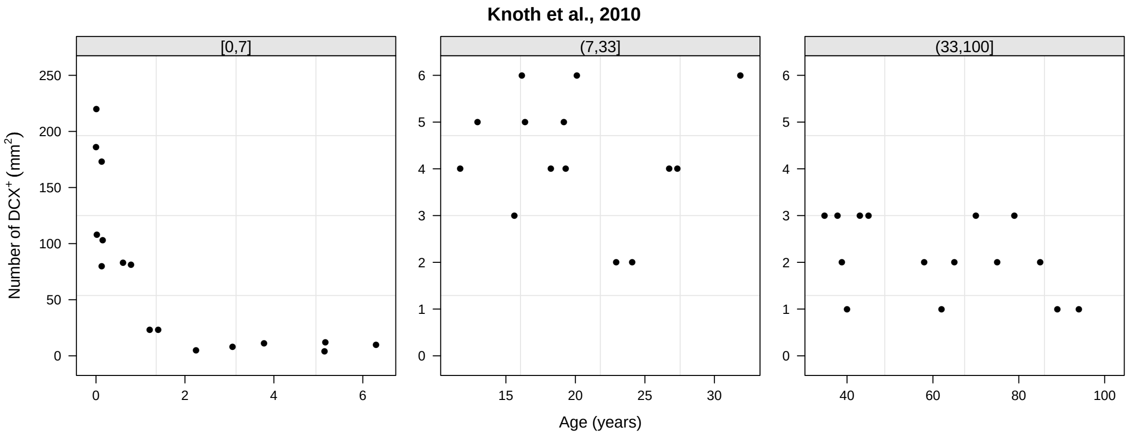


Figure 11: In the bottom 3 panels, the data are plotted separately for ages 0–7, 7–33, and 33-100. Note the different $y$-axes.

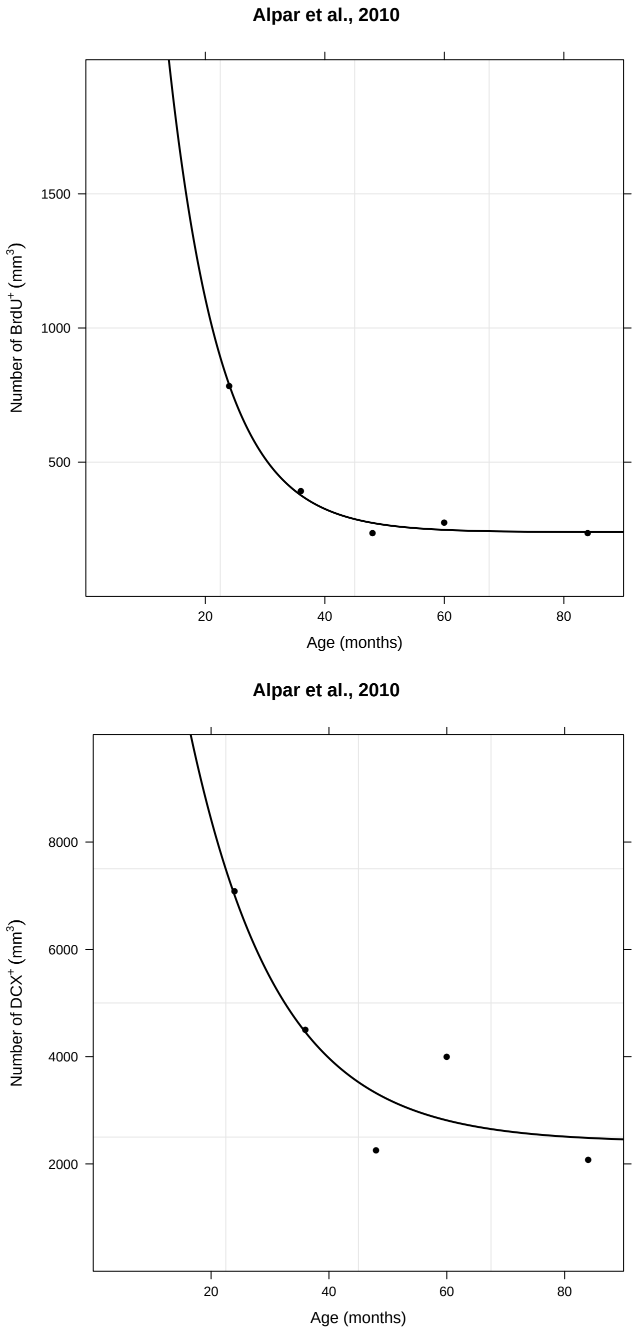
Alpar et al., 2010
Number of BrdU+ (mm3)
1500
1000
500
20
40
60
80
Age (months)
Alpar et al., 2010
Number of DCX+ (mm3)
8000
6000
4000
2000
20
40
60
80
Age (months)

Figure 12:
